# Supplementary material for: A constructive solution to the cosmological bootstrap
Source: arXiv:2305.08939 source file (2023-06-27)
Supplement: Supplementary file 1 [file Appendix_6j.tex]

%%%%%%%%%%%%%%%%%%%%%%%%%%%%%%%%%%%%%%%%%%%%%%%%%%%%%%%%%%%%%%%%%%%%%%%%%%%%%%%%%
\section{Basics of 6j symbols}
\label{sec:6jbasics}
%%%%%%%%%%%%%%%%%%%%%%%%%%%%%%%%%%%%%%%%%%%%%%%%%%%%%%%%%%%%%%%%%%%%%%%%%%%%%%%%%
